# Supplementary material for: A density Corr\'adi-Hajnal Theorem
Source: arXiv:1403.3837 ancillary file (2014-07-30)
Supplement: Supplementary file 1 [file computerverification.pdf]

In this sheet, we verify some of the lengthier computations from the paper "A DENSITY CORRADI-HAJNAL THEOREM".
In Cells 1-5 we introduce quantities needed to this end.
The proof of Lemma 9 is supported by Cells 6 and 7.
The proof of Lemma 17 is supported by Cells 8 and 9.
The calculations from the beginning of the Appendix (page 30) go from Cell 10 to Cell 18.
The support for the proof of Lemma 23 ranges from Cell 19 to Cell 24.
The support of the proof of Lemma 19 ranges from Cell 25 to Cell 34.
The support for the proof of Lemma 20 ranges from Cell 35 to Cell 72.

# Preliminaries

In Cells 1-4 we define functions e_1(n,k), ..., e_4(n,k) corresponding to e(E_1(n,k)),...,e(E_4(n,k)), respectively.
The formulas are taken from (2) on page 5.

```
(%i1) e_1(n,k) :=
      binomial(k,2)+k*(n-k)+ceiling((n-k)/2)*floor((n-k)/2);
```

(%o1) $$e\_1(n,k):=\binom{k}{2}+k\,(n-k)+\mathrm{ceiling}\left(\frac{n-k}{2}\right)\mathrm{floor}\left(\frac{n-k}{2}\right)$$

```
(%i2) e_2(n,k):=
      binomial(2*k+1,2)+ceiling(n/2)*floor(n/2);
```

(%o2) $$e\_2(n,k):=\binom{2\,k+1}{2}+\mathrm{ceiling}\left(\frac{n}{2}\right)\mathrm{floor}\left(\frac{n}{2}\right)$$

```
(%i3) e_3(n,k):=
      binomial(2*k+1,2)+(2*k+1)*(n-2*k-1);
```

(%o3) $$e\_3(n,k):=\binom{2\,k+1}{2}+(2\,k+1)\,(n-2\,k-1)$$

```
(%i4) e_4(n,k):=
      binomial(6*k-n+4,2)+(6*k-n+4)*(n-3*k-2)+(n-3*k-2)^2;
```

(%o4) $$e\_4(n,k):=\binom{6\,k-n+4}{2}+(6\,k-n+4)\,(n-3\,k-2)+(n-3\,k-2)^2$$

In Cell 5 we define the function F which corresponds to the function f' in Equation (3) on page 13. The reason for this change in notation is that Maxima does not allow the symbol '.

```
(%i5) F(t_1,t_2,t_3,t_4,m,i):=
        4*m*t_1+2*i*t_1+7*binomial(t_1,2)+3*t_1+2*i*t_2
        + 8*binomial(t_2,2)+3*t_2 +8*binomial(t_3,2)+8*t_3*t_4+3*t_3
        + 7*t_1*t_2+(2+3*m)*t_2 +7*t_1*(t_3+t_4)
        +(3+3*m)*t_3+8*t_2*(t_3+t_4)+(2+i)*t_3;
```

(%o5) $$F(t\_1,t\_2,t\_3,t\_4,m,i):=4\,m\,t\_1+2\,i\,t\_1+7\binom{t\_1}{2}+3\,t\_1+2\,i\,t\_2+8\binom{t\_2}{2}+3\,t\_2+8\binom{t\_3}{2}+8\,t\_3\,t\_4+3\,t\_3+7\,t\_1\,t\_2+(2+3\,m)\,t\_2+7\,t\_1\,(t\_3+t\_4)+(3+3\,m)\,t\_3+8\,t\_2\,(t\_3+t\_4)+(2+i)\,t\_3$$

Note that when m>0 and i>0, or when t_2=t_3=0, we have f=f'=F (cf. Equation (4) on page 13).

# Support for the proof of Lemma 9 (page 14)

We define H as in Equation (8) from page 14. This definition is incorrect when m=0 or i=0. However, the function h is used only in Cell 7, where the remaining cases are treated seperately.

```
(%i6) H(t_1,t_2,t_3,t_4,m,i):=F(t_1,t_2,t_3,t_4,m,i)+i*m+m^2
      +(3+3*m)*t_4+(2+i)*t_4+binomial(3*t_4,2);
```

(%o6) $H(t\_1,t\_2,t\_3,t\_4,m,i):=F(t\_1,t\_2,t\_3,t\_4,m,i)+i\,m+m^2+(3+3\,m)\,t\_4+(2+i)\,t\_4+\binom{3\,t\_4}{2}$

We verify Equation (9) from page 14. This is done by subtracting the right-hand side of the equation.
In the case m>0 and i>0 the functions H and h are identical.
In the case when m=0 or i=0, the difference between H and h nullifies.
This is because the difference between f and f' depends only on the second and the third coordinate, and these coordinates are identical in the two occurences below.

```
(%i7) expand(H(t_1+t_3+t_4,t_2,0,0,m,i)-H(t_1,t_2,0,t_3+t_4,m,i)
      -(t_3+t_4)*(m+i-t_2-t_3-t_4-4));
```

(%o7) 0

End of the support for the proof of Lemma 9.

# Support for the proof of Lemma 17 (page 26)

Case when 2 < a <= h/9 (middle of page 27)

We define the function p(h,a) by Equation (14) on page 22 for 9a<=h.

```
(%i8) p(h,a):=(a-2)*(h-a+2)+binomial(h-2*a+4,2);
```

(%o8) $p(h,a):=(a-2)\,(h-a+2)+\binom{h-2\,a+4}{2}$

We verify Equation (21) from page 27 by subtracting the right-hand side.

```
(%i9) expand(binomial(h-6-2*(a-2),2)+(a-2)*(h-6-(a-2))
      +2*h-6*a-9+4*h-p(h,a));
```

(%o9) 0

End of the support for the proof of Lemma 17.

# Calculations from page 31

We verify Equation (22) from page 31 for the case m>0 by subtracting the right-hand side. For the case m>0, i>0, we can use F=f' instead of f.

```
(%i10) expand(F(t_1+x,t_2-x,t_3,t_4,m,i)-F(t_1,t_2,t_3,t_4,m,i)
       -(x^2/2+(m-t_2-t_3-t_4+1/2)*x-2*x));
```

```
(%o10) 0
```

For the case when m>0 and i=0

```
(%i11) expand((F(t_1+x,t_2-x,t_3,t_4,m,i)-2*t_3)
       -(F(t_1,t_2,t_3,t_4,m,i)-2*t_3)
       -(x^2/2+(m-t_2-t_3-t_4+1/2)*x-2*x));
```

```
(%o11) 0
```

For the case when m=0 and i>0

```
(%i12) expand(F(t_1+x,t_2-x,t_3,t_4,m,i)-(2*(t_2-x)+3*t_3)
       -(F(t_1,t_2,t_3,t_4,m,i)-(2*(t_2)+3*t_3))
       -(x^2/2+(m-t_2-t_3-t_4+1/2)*x));
```

```
(%o12) 0
```

Finally the case when m=0 and i=0

```
(%i13) expand(F(t_1+x,t_2-x,t_3,t_4,m,i)-(2*(t_2-x)+5*t_3)-
       (F(t_1,t_2,t_3,t_4,m,i)-(2*(t_2)+5*t_3))
       -(x^2/2+(m-t_2-t_3-t_4+1/2)*x));
```

```
(%o13) 0
```

We verify Inequality (23) from page 30 by subtracting the right-hand side of the inequality and obtaining a non-negative term. For m>0 and i>0 we can use F=f' instead of f.

```
(%i14) expand(F(t_1,t_2+t_3,0,t_4,m,i)-F(t_1,t_2,t_3,t_4,m,i)
       -((i-3)*t_3));
```

```
(%o14) 0
```

For m=0 and i>0

```
(%i15) expand(F(t_1,t_2+t_3,0,t_4,m,i)-(2*(t_2+t_3)+3*0)
       -(F(t_1,t_2,t_3,t_4,m,i)-(2*t_2+3*t_3))-((i-3)*t_3));
```

(%o15) $t_3$

for m>0 and i=0

```
(%i16) expand(F(t_1,t_2+t_3,0,t_4,m,i)-(2*0)-(F(t_1,t_2,t_3,t_4,m,i)
       -(2*t_3))-((i-3)*t_3));
```

(%o16) $2\,t_3$

and for m=0 and i=0

```
(%i17) expand(F(t_1,t_2+t_3,0,t_4,m,i)-(2*(t_2+t_3)+5*0)
       -(F(t_1,t_2,t_3,t_4,m,i)-(2*t_2+5*t_3))-((i-3)*t_3));
```

(%o17) $3\,t_3$

We verify Inequality (25) from page 31 by subtracting the
right-hand side. We can use F=f' instead of f in cases that the
last two parameters of the function f are strictly positive. The difference
f'-f compensates in the two appearences when the pairs (m-x,i+2*x) and (m,i)
have the same pair of signs (same as in the remark prior to Cell 7).
In that case, we have

```
(%i18) expand(F(t_1,t_2,t_3,t_4,m-x,i+2*x)-F(t_1,t_2,t_3,t_4,m,i)
       -(x*(t_2-t_3)));
```

```
(%o18) 0
```

By the assumptions min(m,m-x,i+2*x)>0, i=>0, x=>0, the only case when
this does not happen is when (m-x,i+2*x) has signs (+,+) and (m,i) has
signs (+,0). It can be verified that in that case, the inequality is strict.

# Support for the proof of Lemma 23 (page 31)

Part iii):
We verify Equation (27) from page 31.
First, we verify the equality between the first and the second line,
by subtracting them and substituting i by n-3k-2m.

```
(%i19) expand(subst(n-3*k-2*m,i,F(k,0,0,0,m,i)+i*m+m^2
       -(7*binomial(k,2)+3*k+2*(n-3*k)*k+m*(n-3*k-m))));
```

```
(%o19) 0
```

Further, we compare the third and fourth lines.

```
(%i20) expand(7*binomial(k,2)+3*k+2*(n-3*k)*k
       +(floor((n-k)/2)-k)*(ceiling((n-k)/2)-k)
       -(binomial(k,2)+k*(n-k)+floor((n-k)/2)*ceiling((n-k)/2)));
```

(%o20) $k\,n-k\,\mathrm{floor}\left(\frac{n}{2}-\frac{k}{2}\right)-k\,\mathrm{ceiling}\left(\frac{n}{2}-\frac{k}{2}\right)-k^2$

In the above, we use that floor(n/2-k/2)+ceiling(n/2-k/2)=n-k.
Thus %o20 equals to 0.

We verify Equation (28) from page 33. First we compare the
first and second line. Note that
f(t_1,t_2,0,t_4,0,i)=f'(t_1,t_2,0,t_4,0,i)-2t_2=F(t_1,t_2,0,t_4,0,i)-2t_2.

```
(%i21) expand(F(0,k,0,0,0,n-3*k)-2*k-(2*(n-3*k)*k+8*binomial(k,2)+3*k));
```

```
(%o21) 0
```

We compare the third and fourth line. Note that
f(0,k,0,0,1,n-3*k-2)=f'(0,k,0,0,1,n-3*k-2)=F(0,k,0,0,1,n-3*k-2).

```
(%i22) expand(8*binomial(k,2)+2*(n-3*k-2)*k+3*k+5*k-F(0,k,0,0,1,n-3*k-2));
```

```
(%o22) 0
```

We verify Equation (29) from page 33 by subtracting the
second line from the LHS of the first line.
As above, in this range we have f=F=f'.

We substitute n by 3k+2m+i.

```
(%i23) expand(subst(3*k+2*m+i,n,F(0,k,0,0,m,i)+i*m+m^2
       -(8*binomial(k,2)+5*k+2*(n-3*k)*k+m*(n-m-4*k))));
```

(%o23) 0

We verify Equation (30) from page 33 by subtracting the
right-hand side.
Again, in this range we have f=F=f'.

```
(%i24) expand(F(0,k,0,0,1,n-3*k-2)+ (n-3*k-2)*1+1^2-e_3(n,k));
```

(%o24) 0

End of the support of the proof of Lemma 23.

# Support for the proof of the Lemma 19 (page 34)

The function g_s is defined in Equation (15) from page 23.
Here we use G_s, a modified version of g_s, using F=f' instead of f.
Note that G_s=g_s, when m>0 and i>0.

```
(%i25) G_s(t_1,t_2,t_3,t_4,m,i):= F(t_1,t_2,t_3,t_4,m,i) +i*m+m^2
       +(3+3*m)*t_4+(2+i)*t_4+8*binomial(t_4,2)+10*t_4-28;
```

(%o25) $G\_s(t\_1,t\_2,t\_3,t\_4,m,i):=F(t\_1,t\_2,t\_3,t\_4,m,i)+i\,m+m^2+(3+3\,m)\,t\_4+(2+i)\,t\_4+8\binom{t\_4}{2}+10\,t\_4-28$

We verify Inequality (31) from page 34 by subtracting the
right-hand side and obtaining a non-positive term.
For m>0 and i>0, G_s=g_s and we get:

```
(%i26) expand(G_s(t_1,t_2,t_3,t_4,m,i)-G_s(t_1,t_2+t_3+t_4,0,0,m,i)
       -(9*t_4-(t_3+t_4)*(i-3)));
```

(%o26) $-2\,t\_4$

for m=0 and i>0:

```
(%i27) expand(G_s(t_1,t_2,t_3,t_4,m,i)-(2*t_2+3*t_3)
       -(G_s(t_1,t_2+t_3+t_4,0,0,m,i)-(2*(t_2+t_3+t_4)+3*0))
       -(9*t_4-(t_3+t_4)*(i-3)));
```

(%o27) $-t\_3$

for m>0 and i=0:

```
(%i28) expand(G_s(t_1,t_2,t_3,t_4,m,i)-(2*t_3)
       -(G_s(t_1,t_2+t_3+t_4,0,0,m,i)-(2*0))
       -( 9*t_4-(t_3+t_4)*(i-3)));
```

(%o28) $-2\,t\_4-2\,t\_3$

and for m=0 and i=0:

(%i29) expand(G_s(t_1,t_2,t_3,t_4,m,i)-(2*t_2+5*t_3)
-(G_s(t_1,t_2+t_3+t_4,0,0,m,i)-(2*(t_2+t_3+t_4)+5*0))
-( 9*t_4-(t_3+t_4)*(i-3)));

(%o29) $-3\, t\_3$

In Inequality (33) from page 35 we compare the second and third lines.

(%i30) expand(subst(k,t_1+t_2+t_3+t_4,8*binomial(t_1+t_2+t_3+t_4,2)
+(4*m+2*i+15)*(t_1+t_2+t_3+t_4)-28+i*m+m^2
-(8*binomial(k,2)+2*k*(n-3*k)+20*k+((n-3*k)/2)^2)));

(%o30) $4\, k\, t\_4+4\, k\, t\_3+4\, k\, t\_2+4\, k\, t\_1-\frac{n^2}{4}-\frac{k\, n}{2}+m^2+4\, k\, m+i\, m-\frac{k^2}{4}+2\, i\, k-5\, k-28$

(%i31) expand(subst(3*k+2*m+i,n,%o30));

(%o31) $4\, k\, t\_4+4\, k\, t\_3+4\, k\, t\_2+4\, k\, t\_1-4\, k^2-5\, k-\frac{i^2}{4}-28$

As 4*k*t_4+4*k*t_3+4*k*t_2+4*k*t_1=4*k^2, the above is negative.

We verify Inequality (35) from page 35 by subtracting the penultimate term. When m-25>0 and i>0, the two occurences of the function g_s in (35) coincide with G_s. By assumption m-25>0. If i=0, the difference between g_s and G_s depends on the third coordinate, which is 0. Thus, g_s()-g_s()=G_s()-G_s().

(%i32) expand(subst(t_1+t_2+t_3+t_4,k,G_s(t_1,k-t_1,0,0,m-25,i+50)
-G_s(t_1,k-t_1,0,0,m,i)-(12*(k-t_1))));

(%o32) $13\, t\_4+13\, t\_3+13\, t\_2-25\, i-625$

As i<12, and t_2+t_3+t_4>80, the above is positive.

We verify Inequality (36) from page 36 by subtracting the right hand-side. If m>0 and i>0, we have G_s=g_s.
As the third coordinate is the same in both functions, we obtain the same result even when m>0 and i=0.

(%i33) expand(G_s(k,0,0,0,m,i)-G_s(t_1,k-t_1,0,0,m,i)-((k-t_1)*m
-binomial(k-t_1,2)-2*(k-t_1)));

(%o33) 0

If m=0, we get

(%i34) expand(G_s(k,0,0,0,m,i)-(2*0+0)
-(G_s(t_1,k-t_1,0,0,m,i)-(2*(k-t_1)+0))
-((k-t_1)*m-binomial(k-t_1,2)-2*(k-t_1)));

(%o34) $2\, k-2\, t\_1$

Which is non-negative.

End of the support of the proof of Lemma 19.

# Support for the proof of Lemma 20

# (page 36)

Case 1: 3t_430

We define the auxiliary function h from Equation (37)
from page 37:

(%i35) h(t_1,t_2,t_3,t_4,m,i):=4*m*t_1+2*i*t_1+7*binomial(t_1,2)
+3*t_1+2*i*t_2+8*binomial(t_2,2)+3*t_2+8*binomial(t_3,2)
+8*t_3*t_4+3*t_3+7*t_1*t_2+(2+3*m)*t_2+7*t_1*(t_3+t_4)
+(3+3*m)*t_3+8*t_2*(t_3+t_4)+(2+i)*t_3+i*m+m^2+(3+3*m)*t_4+
(2+i)*t_4+binomial(3*t_4,2);

(%o35) $h(t\_1,t\_2,t\_3,t\_4,m,i):=4\,m\,t\_1+2\,i\,t\_1+7\binom{t\_1}{2}+3\,t\_1+2\,i\,t\_2+8\binom{t\_2}{2}+3\,t\_2+8\binom{t\_3}{2}+8\,t\_3\,t\_4+3\,t\_3+7\,t\_1\,t\_2+(2+3\,m)\,t\_2+7\,t\_1\,(t\_3+t\_4)+(3+3\,m)\,t\_3+8\,t\_2\,(t\_3+t\_4)+(2+i)\,t\_3+i\,m+m^2+(3+3\,m)\,t\_4+(2+i)\,t\_4+\binom{3\,t\_4}{2}$

We verify the following equations [Equations (38), (39), (40)]
from page 37:

(%i36) expand(h(t_1+x,t_2,t_3,t_4-x,m,i)-h(t_1,t_2,t_3,t_4,m,i));

(%o36) $x^2-2\,t\_4\,x-t\_3\,x-t\_2\,x+m\,x+i\,x-4\,x$

(%i37) expand(h(t_1,t_2+x,t_3,t_4-x,m,i)-h(t_1,t_2,t_3,t_4,m,i));

(%o37) $\frac{x^2}{2}-t\_4\,x+i\,x-\frac{5\,x}{2}$

(%i38) expand(h(t_1,t_2,t_3+x,t_4-x,m,i)-h(t_1,t_2,t_3,t_4,m,i));

(%o38) $\frac{x^2}{2}-t\_4\,x+\frac{x}{2}$

We verify the following equations [Equation (41), (42), (43)] from page 37.

(%i39) expand(h(t_1+x,t_2,t_3-x,t_4,m,i)-h(t_1,t_2,t_3,t_4,m,i));

(%o39) $\frac{x^2}{2}-t\_4\,x-t\_3\,x-t\_2\,x+m\,x+i\,x-\frac{9\,x}{2}$

(%i40) expand(h(t_1+x,t_2-x,t_3,t_4,m,i)-h(t_1,t_2,t_3,t_4,m,i));

(%o40) $\frac{x^2}{2}-t\_4\,x-t\_3\,x-t\_2\,x+m\,x-\frac{3\,x}{2}$

(%i41) expand(h(t_1,t_2+x,t_3-x,t_4,m,i)-h(t_1,t_2,t_3,t_4,m,i));

(%o41) $i\,x-3\,x$

Next, we want to verify Equation (44) from page 37.
As t_4<(n-3k)/3=(2m+i)/3, the function g_l is defined by
Equation (16) from page 23. For simplification, we modify slightly
the definition of g_l using f'=F instead of f. In the following, we argue
that it does not affect the result.

(%i42) g_l(t_1,t_2,t_3,t_4,m,i):=F(t_1,t_2,t_3,t_4,m,i)+i*m+m^2
+(3+3*m)*t_4+(2+i)*t_4+binomial(3*t_4,2);

(%o42) $g\_l(t\_1,t\_2,t\_3,t\_4,m,i):=F(t\_1,t\_2,t\_3,t\_4,m,i)+i\,m+m^2+(3+3\,m)\,t\_4+(2+i)\,t\_4+\binom{3\,t\_4}{2}$

We verify Equation (44) from page 37: here t_3=t_4=0 and therefore f=f'=F. This implies we can use the modified definition of g_l and obtain the same result.
First, we expand the lef-hand side.

(%i43) expand(g_l(k,0,0,0,m,i)-g_l(2*k-n/3,0,0,(n-3*k)/3,m,i));

(%o43) $-\frac{n^2}{9}+\frac{m\,n}{3}+\frac{2\,k\,n}{3}+\frac{i\,n}{3}-\frac{4\,n}{3}-k\,m-k^2-i\,k+4\,k$

To evaluate the previous equation, we subtract the right-hand side of Equation (44), i.e. we subtract ((n-3k)/3)*((n-3k)/6+i/2-4).
Further, we substitute n by 3k+2m+i.

(%i44) expand(subst(3*k+2*m+i,n,%o43-((n-3*k)*((n-3*k)/6+i/2-4)/3)));

(%o44) 0

To verify Equation (45) from page 38, we subtract the right-hand side of the equation.

(%i45) expand(h(0,2*k-n/3,0,(n-3*k)/3,m,i)-(3*i*k-(i*n)/3+n^2/18-3*k/2
+5*n/6+3*k*m-k*n/3+9*k^2/2+i*m+m^2));

(%o45) 0

To verify Equation (46) from page 38, we subtract the right-hand side and check that we obtain only linear terms.
We substitute i by n-3*k-2*m.

(%i46) expand(subst(n-3*k-2*m,i,h(0,2*k-n/3,0,(n-3*k)/3,m,i)
-(11*k*n/3-9*k^2/2-6*k*m-5*n^2/18+5*m*n/3-m^2)));

(%o46) $\frac{5\,n}{6}-\frac{3\,k}{2}$

Subcase 1: We verify Equations (47) and (48)
from page 38 by subtracting the respective right-hand sides and checking that the result is a linear term.

(%i47) expand(h(0,2*k-n/3,0,(n-3*k)/3,0,n-3*k)-(11*k*n/3-9*k^2/2-5*n^2/18));

(%o47) $\frac{5\,n}{6}-\frac{3\,k}{2}$

(%i48) expand(h(0,2*k-n/3,0,(n-3*k)/3,0,n-3*k)-e_4(n,k)
-(-7*n^2/9+20*k*n/3-27*k^2/2));

(%o48) $\frac{7\,n}{3}-\frac{21\,k}{2}-2$

Subcase 2: In Equation (49) from page 38 we subtract the right-hand sides and verify that we obtain a linear term.

(%i49) expand(h(0,2*k-n/3,0,(n-3*k)/3,0,n-3*k)-e_3(n,k)

-(5*k*n/3-5*k^2/2-5*n^2/18));

(%o49) $-\frac{n}{6}+\frac{3\,k}{2}+1$

Subcase 3: In equations (50) and (51) from page 38
we subtract the respective right-hand sides and verify that the results
are linear.

(%i50) expand(h(0,2*k-n/3,0,(n-3*k)/3,5*n/6-3*k,3*k-2*n/3)
-(-4*k*n/3+9*k^2/2+15*n^2/36));

(%o50) $\frac{5\,n}{6}-\frac{3\,k}{2}$

(%i51) expand(h(0,2*k-n/3,0,(n-3*k)/3,5*n/6-3*k,3*k-2*n/3)-e_3(n,k)
-(-10*k*n/3+13*k^2/2+15*n^2/36));

(%o51) $-\frac{n}{6}+\frac{3\,k}{2}+1$

Subcase 4: In equations (52) and (53) from page 38,
again we subtract the respective right-hand sides and obtain a linear term.

(%i52) expand(h(0,2*k-n/3,0,(n-3*k)/3,(n-3*k)/2,0)
-(-k*n/3+11*n^2/36+9*k^2/4));

(%o52) $\frac{5\,n}{6}-\frac{3\,k}{2}$

(%i53) expand(h(0,2*k-n/3,0,(n-3*k)/3,(n-3*k)/2,0)-e_1(n,k)
-(5*k^2/2-5*k*n/6+n^2/18));

(%o53) $\frac{n^2}{4}-\frac{k\,n}{2}+\frac{5\,n}{6}-\mathrm{ceiling}\left(\frac{n}{2}-\frac{k}{2}\right)\,\mathrm{floor}\left(\frac{n}{2}-\frac{k}{2}\right)+\frac{k^2}{4}-k$

In the result above, we use that
ceiling(n/2-k/2)*floor(n/2-k/2)≈n^2/4-k*n/2+k^2/4, and see that all
remaining terms are linear.

Case 2: 3t_4>=max(528,3k_0,2m+i)

We define the function h [Equation (54)] from page 39:

(%i54) h(t_1,t_2,t_3,t_4,m,i):=4*m*t_1+2*i*t_1+7*binomial(t_1,2)
+3*t_1+2*i*t_2+8*binomial(t_2,2)+3*t_2+8*binomial(t_3,2)
+8*t_3*t_4+3*t_3+7*t_1*t_2+(2+3*m)*t_2+7*t_1*(t_3+t_4)
+(3+3*m)*t_3+8*t_2*(t_3+t_4)+(2+i)*t_3+(2*m+i-2)*(3*t_4+2)
+binomial(3*t_4-2*m-i+4,2);

(%o54) $\mathrm{h}(t\_1,t\_2,t\_3,t\_4,m,i):=4\,m\,t\_1+2\,i\,t\_1+7\binom{t\_1}{2}+3\,t\_1+2\,i\,t\_2+8\binom{t\_2}{2}+3\,t\_2+8\binom{t\_3}{2}+8\,t\_3\,t\_4+3\,t\_3+7\,t\_1\,t\_2+(2+3\,m)\,t\_2+7\,t\_1\,(t\_3+t\_4)+(3+3\,m)\,t\_3+8\,t\_2\,(t\_3+t\_4)+(2+i)\,t\_3+(2\,m+i-2)\,(3\,t\_4+2)+\binom{3\,t\_4-2\,m-i+4}{2}$

We verify Equation (55) from page 39

(%i55) expand(h(t_1+x,t_2-x,t_3,t_4,m,i)-h(t_1,t_2,t_3,t_4,m,i));

(%o55) $\frac{x^2}{2}-t\_4\,x-t\_3\,x-t\_2\,x+m\,x-\frac{3\,x}{2}$

Equation (56)

(%i56) expand(h(t_1+x,t_2,t_3-x,t_4,m,i)-h(t_1,t_2,t_3,t_4,m,i));

(%o56) $\frac{x^2}{2}-t\_4\,x-t\_3\,x-t\_2\,x+m\,x+i\,x-\frac{9\,x}{2}$

Equation (57)

(%i57) expand(h(t_1,t_2+x,t_3-x,t_4,m,i)-h(t_1,t_2,t_3,t_4,m,i));

(%o57) $i\,x-3\,x$

Equation (58)

(%i58) expand(h(t_1+x,t_2,t_3,t_4-x,m,i)-h(t_1,t_2,t_3,t_4,m,i));

(%o58) $x^2-2\,t\_4\,x-t\_3\,x-t\_2\,x+4\,m\,x+2\,i\,x-5\,x$

Equation (59)

(%i59) expand(h(t_1,t_2+x,t_3,t_4-x,m,i)-h(t_1,t_2,t_3,t_4,m,i));

(%o59) $\frac{x^2}{2}-t\_4\,x+3\,m\,x+2\,i\,x-\frac{7\,x}{2}$

and Equation (60).

(%i60) expand(h(t_1,t_2,t_3+x,t_4-x,m,i)-h(t_1,t_2,t_3,t_4,m,i));

(%o60) $\frac{x^2}{2}-t\_4\,x+3\,m\,x+i\,x-\frac{x}{2}$

In Subcase 1 we verify Equation (61) and Equation (62)
from page 39 by subtracting the right-hand side and checking that we get
only linear terms.
We substitute i by n-3k-2m.

(%i61) expand(subst(n-3*k-2*m,i,h(2*k-n/3,0,0,(n-3*k)/3,m,i)
-(7*k*n/3-n^2/18-3*k^2)));

(%o61) $\frac{n}{6}-k+2$

(%i62) expand(subst(n-3*k-2*m,i,h(2*k-n/3,0,0,(n-3*k)/3,m,i)-e_2(n,k)
-(7*k*n/3-11*n^2/36-5*k^2)));

(%o62) $-\mathrm{ceiling}\left(\frac{n}{2}\right)\,\mathrm{floor}\left(\frac{n}{2}\right)+\frac{n^2}{4}+\frac{n}{6}-2\,k+2$

In the above, we use that ceiling(n/2)*floor(n/2)≈n^2/4, and see that
all remaining terms are linear.

In Subcase 2, we verify Equation (63) from page 39 by subtracting
the right-hand side and check we obtain only linear terms.
For that we substitute i by n-3k-2m.

(%i63) expand(subst(n-3*k-2*m,i,h(2*k-n/3,0,0,(n-3*k)/3,m,i)-e_3(n,k)
-(k*n/3-n^2/18-k^2)));

(%o63) $-\frac{5n}{6}+2k+3$

In Subcase 3, we verify Equation (64) from page 40 by subtracting the right-hand side. Again, we substitute i by n-3k-2m.

(%i64) expand(subst(n-3*k-2*m,i,h(0,2*k-n/3,0,(n-3*k)/3,m,i)
-(7*k*n/6+n^2/18+i*(k-n/6)+2*k-n/3+2)));

(%o64) 0

For Equation (65) from page 40, we subtract the right-hand side and verify we get linear terms. We substitute i by n-3k-2m.

(%i65) expand(subst(n-3*k-2*m,i,h(0,2*k-n/3,0,(n-3*k)/3,m,i)-e_2(n,k)
-(8*k*n/3-13*n^2/36-5*k^2)));

(%o65) $-\mathrm{ceiling}\left(\frac{n}{2}\right)\mathrm{floor}\left(\frac{n}{2}\right)+\frac{n^2}{4}+\frac{m\,n}{3}-\frac{n}{3}-2\,k\,m+k+2$

In the above we use that ceiling(n/2)*floor(n/2)≈n^2/4. Further, we have the assumption that i=n-3k, that is m=0. The remaining terms are linear.

In Subcase 4 we verify Equation (66) from page 40. We subtract the right-hand side, substitute i by n-3k-2m and obtain linear terms.

(%i66) expand(subst(n-3*k-2*m,i,h(0,2*k-n/3,0,(n-3*k)/3,m,i)-e_3(n,k)
-(2*k*n/3-n^2/9-k^2)));

(%o66) $\frac{m\,n}{3}-\frac{4\,n}{3}-2\,k\,m+5\,k+3$

In the above, we use the assumption that i=n-3k and thus m=0. The remaining terms are linear.

In Subcase 5, we verify Equation (67) from page 40. We subtract the right-hand side, substitute i by n-3k-2m.

(%i67) expand(subst(n-3*k-2*m,i,h(0,2*k-n/3,0,(n-3*k)/3,m,i)-e_4(n,k)
-(17*k*n/3-11*n^2/18-12*k^2)));

(%o67) $\frac{m\,n}{3}+\frac{7\,n}{6}-2\,k\,m-7\,k$

In the above, we use the assumption that i=n-3k and thus m=0.
The remaining terms are linear.

The assumption k>3n/10 coming from Subcase 5 implies that the function p is used only in this range (in the definition of g_l).

(%i68) p(h,a):=(a-2)*(h-a+2)+binomial(h-2*a+4,2);

(%o68) $\mathrm{p}(h,a):=(a-2)\,(h-a+2)+\binom{h-2\,a+4}{2}$

For t_1=0 or t_1=1, we can define g_l(t_1,0,0,k,m,i) as follows (see Equations (17) and (18) from page 23):

```
(%i69) g_l(t_1):=F(t_1,0,0,k-t_1,m,i)+p(3*(k-t_1)+2*m+i,2*m+i)+20*t_1;
```

(%o69) $g\_l(t\_1):=F(t\_1,0,0,k-t\_1,m,i)+p(3(k-t\_1)+2m+i,2m+i)+20\,t\_1$

We define the right-hand side of Equation (68) from page 40 by RHS(t_1) as follows.

```
(%i70) RHS(t_1):=(2*n-8*k-3/2-5*t_1/2)*t_1-3*n/2+9*k^2+9*k-3*k*n+n^2/2+2
       +20*t_1;
```

(%o70) $RHS(t\_1):=\left(2n-8k+\frac{-3}{2}+\frac{(-5)\,t\_1}{2}\right)t\_1-\frac{3n}{2}+9k^2+9k+(-3)\,k\,n+\frac{n^2}{2}+2+20\,t\_1$

We verify that LHS=RHS in Equation (68) from page 40. In a first step, we substitute n by 3k+2m+i.

```
(%i71) expand(subst(3*k+2*m+i,n,g_l(t_1)-RHS(t_1)));
```

(%o71) $\frac{7\,t\_1^2}{2}-\frac{7\,t\_1}{2}$

The above equals 0 for t_1=0 or t_1=1.

We verify Equation (69) from page 41 by subtracting the right-hand side and substituying n by 3k+2m+i.

```
(%i72) expand(subst(3*k+2*m+i,n,g_l(0)-e_4(n,k)));
```

(%o72) 0

End of the support for the proof of Lemma 20.

---

Created with wxMaxima.
